# Supplementary material for: Insights into star formation and dispersal from the synchronisation of stellar clocks
Source: arXiv:2311.13042 source file (2023-11-21)
Supplement: Supplementary file 1 [file Supplementary_Information.pdf]

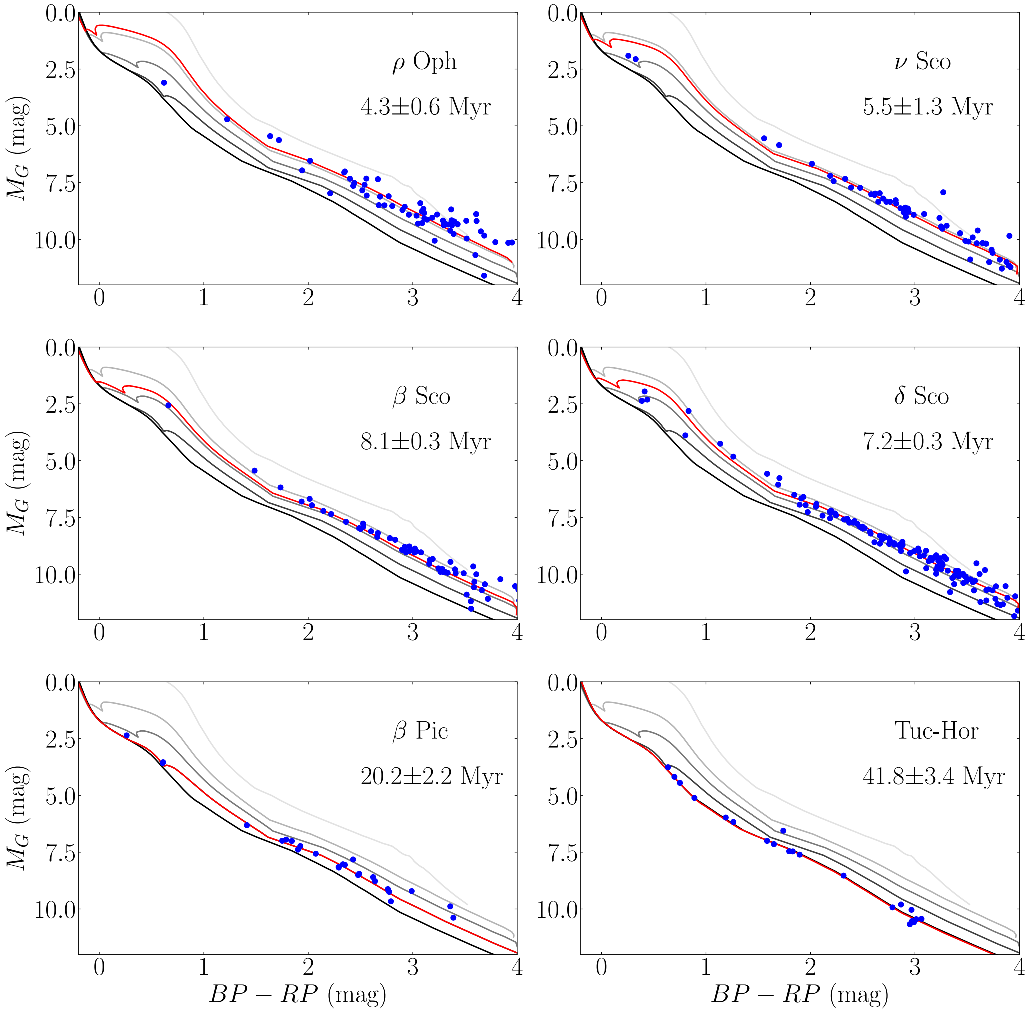


Figure 1: Colour magnitude diagram of the members of the groups considered in this study. The PARSEC isochrones corresponding to the fit computed in this work (using the algorithm[1]) are indicated in red. The PARSEC isochrones at 1, 5, 10, 20, and 40 Myr are also indicated.

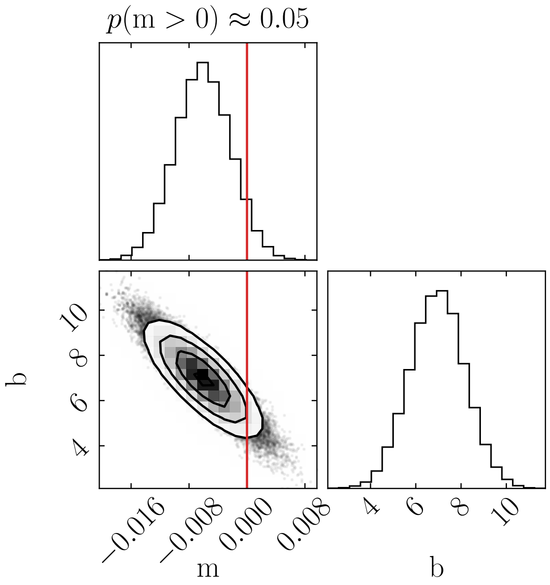


Figure 2: Corner plot showing the posterior PDF of the Bayesian model of the relation between $\Delta_{\mathrm{Age}}$ and the number of association members (Fig. 3). The fit parameters are $m$ (slope) and $b$ (intercept). Diagonal histograms display marginalised parameter distributions and the bottom left panel shows the 2D posterior distribution. The red line indicates the constant relationship ($m = 0$).

Table 1: Literature age estimates for the four regions analysed in this study.

| Region | Method | Age | Reference | Used |
|---|---|---|---|---|
| $\rho$ Oph | Isochrone | $5.7 \pm 0.4$ | Kerr et al. (2021)[2] | Y |
| | | $3.8^{+0.4}_{-0.4}$ | Ratzenböck et al. (2023)[1] | Y |
| | | $4 \pm 1$ | Briceño-Morales et al. (2023)[3] | Y |
| | | $4.3^{+0.6}_{-0.5}$ | **This work** | Y |
| | Kinematics | $0.0 \pm 0.3$ | Miret-Roig et al. (2022)[4] | Y |
| $\nu$ Sco | Isochrone | $7.2 \pm 0.7$ | Kerr et al. (2021)[2] | Y |
| | | $5.8^{+1.8}_{-0.5}$ | Ratzenböck et al. (2023)[1] | Y |
| | | $7 \pm 1$ | Briceño-Morales et al. (2023)[3] | Y |
| | | $5.5^{+1.3}_{-0.4}$ | **This work** | Y |
| | Kinematics | $0.3 \pm 0.5$ | Miret-Roig et al. (2022)[4] | Y |
| $\beta$ Sco | Isochrone | $13.2 \pm 2.8$ | Kerr et al. (2021)[2] | Y |
| | | $7.6^{+0.8}_{-0.7}$ | Ratzenböck et al. (2023)[1] | Y |
| | | $8 \pm 1$ | Briceño-Morales et al. (2023)[3] | Y |
| | | $8.1^{+0.3}_{-0.2}$ | **This work** | Y |
| | Kinematics | $2.5 \pm 1.6$ | Miret-Roig et al. (2022)[4] | Y |
| $\delta$ Sco | Isochrone | $10.2 \pm 0.7$ | Kerr et al. (2021)[2] | Y |
| | | $9.8^{+1.2}_{-1.4}$ | Ratzenböck et al. (2023)[1] | Y |
| | | $9 \pm 2$ | Briceño-Morales et al. (2023)[3] | Y |
| | | $7.2^{+0.3}_{-0.2}$ | **This work** | Y |
| | Kinematics | $4.6 \pm 1.1$ | Miret-Roig et al. (2022)[4] | Y |
| $\beta$ Pic | Isochone | $20 \pm 10$ | Barrado y Navascués et al. (1999b)[5] | N |
| | | $12^{+8}_{-4}$ | Zuckerman et al. (2001)[6] | N |
| | | $21.5 \pm 6.5$ | Malo et al. (2014)[7] | N |
| | | $22 \pm 3$ | Mamajek & Bell (2014)[8] | Y |
| | | $24 \pm 3$ | Bell et al. (2015)[9] | Y |
| | | 5.5 − 54.5 Myr | Ujjwal et al. (2020)[10] | N |
| | | $20.2^{+2.2}_{-1.9}$ | **This work** | Y |
| | Kinematics | 11.5 | Ortega et al. (2002)[11] | N |
| | | 12 | Song et al. (2003)[12] | N |
| | | $10.8 \pm 0.3$ | Ortega et al. (2004)[13] | N |
| | | 18 | Torres et al. (2006)[14] | N |
| | | $31 \pm 21$ | Makarov (2007)[15] | N |
| | | 13 − 58 | Mamajek & Bell (2014)[8] | N |
| | | $13^{+7}_{-0}$ | Miret-Roig et al. (2018)[16] | N |
| | | $17.8 \pm 1.2$ | Crundall et al. (2019)[17] | N |
| | | $18.5^{+2.0}_{-2.4}$ | Miret-Roig et al. (2020)[18] | Y |
| | | $20.4 \pm 2.5$ | Couture et al. (2023)[19] | N |
| | Lithium | $21 \pm 9$ | Mentuch et al. (2008)[20] | N |
| | | $\sim 40$ | Macdonald & Mullan (2010)[21] | N |
| | | $21 \pm 4$ | Binks & Jeffries (2014)[22] | Y |
| | | $26 \pm 3$ | Malo et al. (2014)[7] | Y |
| | | $25 \pm 3$ | Messina et al. (2016)[23] | Y |
| | | $24.3^{+0.3}_{-0.3}$ | Galindo-Guil et al. (2022)[24] | Y |
| | | $22.9^{+1.1}_{-1.0}$ | Jeffries et al. (2023)[25] | Y |
| Tuc-Hor | Isochone | $45 \pm 4$ | Bell et al. (2015)[9] | Y |
| | | $46.3 \pm 2.3$ | Kerr et al. (2022a)[26] | Y |
| | | $41.8^{+3.4}_{-2.2}$ | **This work** | Y |
| | Kinematics | $5^{+23}_{-0}$ | Miret-Roig et al. (2018)[16] | N |
| | | $32.9 \pm 8.2$ | Kerr et al. (2022a)[26] | N |
| | | $38.5^{+1.6}_{-8.0}$ | Galli et al. (2023)[27] | Y |
| | Lithium | $21 \pm 9$ | Mentuch et al. (2008)[20] | N |
| | | $\sim 40$ | Kraus et al. (2014)[28] | N |
| | | $51.0^{+0.5}_{-0.2}$ | Galindo-Guil et al. (2022)[24] | Y |
| | | $41.7^{+3.0}_{-1.9}$ | Jeffries et al. (2023)[25] | Y |

**Notes.** Only the age determinations with an uncertainty $< 5$ Myr were considered for this study, indicated with "Y" in the "Used" column.

## References


1. Ratzenböck, S. *et al.* The star formation history of the Sco-Cen association: Coherent star formation patterns in space and time. *arXiv e-prints* arXiv:2302.07853 (2023).

2. Kerr, R. M. P., Rizzuto, A. C., Kraus, A. L. & Offner, S. S. R. Stars with Photometrically Young Gaia Luminosities Around the Solar System (SPYGLASS). I. Mapping Young Stellar Structures and Their Star Formation Histories. *Astrophys. J.* **917**, 23 (2021).

3. Briceño-Morales, G. & Chanamé, J. Substructure, supernovae, and a time-resolved star formation history for Upper Scorpius. *Mon. Not. R. Astron. Soc.* **522**, 1288–1309 (2023).

4. Miret-Roig, N. *et al.* The star formation history of Upper Scorpius and Ophiuchus. A 7D picture: positions, kinematics, and dynamical traceback ages. *Astron. Astrophys.* **667**, A163 (2022).

5. Barrado y Navascués, D., Stauffer, J. R., Song, I. & Caillault, J.-P. The Age of $\beta$ Pictoris. *Astrophys. J. Lett.* **520**, L123–L126 (1999).

6. Zuckerman, B., Song, I., Bessell, M. S. & Webb, R. A. The $\beta$ Pictoris Moving Group. *Astrophys. J. Lett.* **562**, L87–L90 (2001).

7. Malo, L. *et al.* BANYAN. IV. Fundamental Parameters of Low-mass Star Candidates in Nearby Young Stellar Kinematic Groups—Isochronal Age Determination using Magnetic Evolutionary Models. *Astrophys. J.* **792**, 37 (2014).

8. Mamajek, E. E. & Bell, C. P. M. On the age of the $\beta$ Pictoris moving group. *Mon. Not. R. Astron. Soc.* **445**, 2169–2180 (2014).

9. Bell, C. P. M., Mamajek, E. E. & Naylor, T. A self-consistent, absolute isochronal age scale for young moving groups in the solar neighbourhood. *Mon. Not. R. Astron. Soc.* **454**, 593–614 (2015).

10. Ujjwal, K., Kartha, S. S., Mathew, B., Manoj, P. & Narang, M. Analysis of Membership Probability in Nearby Young Moving Groups with Gaia DR2. *Astron. J.* **159**, 166 (2020).

11. Ortega, V. G., de la Reza, R., Jilinski, E. & Bazzanella, B. The Origin of the $\beta$ Pictoris Moving Group. *Astrophys. J. Lett.* **575**, L75–L78 (2002).

12. Song, I., Zuckerman, B. & Bessell, M. S. New Members of the TW Hydrae Association, $\beta$ Pictoris Moving Group, and Tucana/Horologium Association. *Astrophys. J.* **599**, 342–350 (2003).

13. Ortega, V. G., de la Reza, R., Jilinski, E. & Bazzanella, B. New Aspects of the Formation of the $\beta$ Pictoris Moving Group. *Astrophys. J.* **609**, 243–246 (2004).

14. Torres, C. A. O. *et al.* Search for associations containing young stars (SACY). I. Sample and searching method. *Astron. Astrophys.* **460**, 695–708 (2006).

15. Makarov, V. V. Unraveling the Origins of Nearby Young Stars. *Astrophys. J. Suppl. Ser.* **169**, 105–119 (2007).

16. Miret-Roig, N., Antoja, T., Romero-Gómez, M. & Figueras, F. Dynamical ages of the young local associations with Gaia. *Astron. Astrophys.* **615**, A51 (2018).

17. Crundall, T. D. *et al.* Chronostar: a novel Bayesian method for kinematic age determination - I. Derivation and application to the $\beta$ Pictoris moving group. *Mon. Not. R. Astron. Soc.* **489**, 3625–3642 (2019).

18. Miret-Roig, N. *et al.* Dynamical traceback age of the $\beta$ Pictoris moving group. *Astron. Astrophys.* **642**, A179 (2020).

19. Couture, D., Gagné, J. & Doyon, R. Addressing Systematics in the Traceback Age of the $\beta$ Pictoris Moving Group. *arXiv e-prints* arXiv:2302.04348 (2023).

20. Mentuch, E., Brandeker, A., van Kerkwijk, M. H., Jayawardhana, R. & Hauschildt, P. H. Lithium Depletion of Nearby Young Stellar Associations. *Astrophys. J.* **689**, 1127–1140 (2008).

21. Macdonald, J. & Mullan, D. J. Magneto-convection and Lithium Age Estimates of the $\beta$ Pictoris Moving Group. *Astrophys. J.* **723**, 1599–1606 (2010).

22. Binks, A. S. & Jeffries, R. D. A lithium depletion boundary age of 21 Myr for the Beta Pictoris moving group. *Mon. Not. R. Astron. Soc.* **438**, L11–L15 (2014).

23. Messina, S. *et al.* The rotation-lithium depletion correlation in the $\beta$ Pictoris association and the LDB age determination. *Astron. Astrophys.* **596**, A29 (2016).

24. Galindo-Guil, F. J. *et al.* Lithium depletion boundary, stellar associations, and Gaia. *Astron. Astrophys.* **664**, A70 (2022).

25. Jeffries, R. D. *et al.* The Gaia-ESO Survey: empirical estimates of stellar ages from lithium equivalent widths (EAGLES). *Mon. Not. R. Astron. Soc.* **523**, 802–824 (2023).

26. Kerr, R. *et al.* SPYGLASS. III. The Fornax-Horologium Association and Its Traceback History within the Austral Complex. *Astrophys. J.* **941**, 143 (2022).

27. Galli, P. A. B., Miret-Roig, N., Bouy, H., Olivares, J. & Barrado, D. Dynamical age of the Tucana-Horologium young stellar association. *Mon. Not. R. Astron. Soc.* **520**, 6245–6255 (2023).

28. Kraus, A. L., Shkolnik, E. L., Allers, K. N. & Liu, M. C. A Stellar Census of the Tucana-Horologium Moving Group. *Astron. J.* **147**, 146 (2014).
